# Supplementary material for: Time-Dependent Coupled-Cluster Theory of Multireference Systems
Source: arXiv:2505.04716 ancillary file (2025-05-07)
Supplement: Supplementary file 1 [file si.pdf]

# Supplemental Material: Time-Dependent Coupled-Cluster Theory of Multireference Systems

Martín A. Mosquera[1,*]

[1]*Department of Chemistry and Biochemistry, Montana State University, Bozeman, MT 59717, USA*

[*] martinmosquera@montana.edu

## I. FREQUENCIES, T-AMPLITUDES, SINGULAR VALUES, AND DIPOLES

TABLE I. Comparison between Full MRCI (FMRCI) reference frequencies and EOM-MRCC frequencies for all spin symmetries, singular values, $t$ values, and $\Lambda_0$ values. All numbers are presented in atomic units.

| Index | FMRCI frequencies | EOM-MRCC freqs. | Singular Values | $t$ values | $\Lambda_0$ values |
|---|---|---|---|---|---|
| 1 | 0.026316205599049 | 0.026316205599049 | 1.357876653 | 0.064666821 | 0.051241862 |
| 2 | 0.030559489239818 | 0.030559489239825 | 1.357876653 | 0 | 0 |
| 3 | 0.062694133452408 | 0.062694133452407 | 1.357876653 | 0 | 0 |
| 4 | 0.066030372526388 | 0.066030372526388 | 1.357876653 | 0.079853683 | 0.063908752 |
| 5 | 0.067144864038812 | 0.067144864038813 | 1.166250223 | 0 | 0 |
| 6 | 0.067292070528504 | 0.067292070528505 | 1.166250223 | 0 | 0 |
| 7 | 0.073635604290683 | 0.073635604290689 | 1.166250223 | 0.079853683 | 0.063908752 |
| 8 | 0.101621509342031 | 0.101621509342044 | 1.166250223 | 0 | 0 |
| 9 | 0.101837073380565 | 0.101837073380569 | 1.166250223 | 0 | 0 |
| 10 | 0.103057543882225 | 0.103057543882227 | 1.166250223 | 0 | 0 |
| 11 | 0.103080594796718 | 0.103080594796720 | 1.166250223 | 0 | 0 |
| 12 | 0.104234935022644 | 0.104234935022644 | 1.166250223 | 0 | 0 |
| 13 | 0.105639775496541 | 0.105639775496553 | 1 | 0 | 0 |
| 14 | 0.129540659503773 | 0.129540659503775 | 1 | 0 | 0 |
| 15 | 0.130713598678016 | 0.130713598678015 | 1 | 0 | 0 |
| 16 | 0.131406771880188 | 0.131406771880189 | 1 | 0.088861287 | 0.09638833 |
| 17 | 0.133535497114829 | 0.133535497114833 | 0.939373727 | -0.041268007 | -0.048678072 |
| 18 | 0.133765195775079 | 0.133765195775076 | 0.939373727 | 0 | 0 |
| 19 | 0.134521064341247 | 0.134521064341252 | 0.939373727 | 0 | 0 |
| 20 | 0.147853339243084 | 0.147853339243083 | 0.939373727 | -0.02799735 | -0.030945855 |
| 21 | 0.150723152811352 | 0.150723152811350 | 0.931382524 | 0 | 0 |
| 22 | 0.176443247724811 | 0.176443247724809 | 0.931382524 | 0.153841004 | 0.157755959 |
| 23 | 0.176905668480196 | 0.176905668480202 | 0.931382524 | 0 | 0 |
| 24 | 0.178411156958384 | 0.178411156958384 | 0.931382524 | 0 | 0 |
| 25 | 0.178501940042964 | 0.178501940042965 | 0.79908041 | 0 | 0 |
| 26 | 0.179652259695482 | 0.179652259695482 | 0.79908041 | 0 | 0 |
| 27 | 0.180306549561209 | 0.180306549561212 | 0.79908041 | 0 | 0 |
| 28 | 0.214202301601445 | 0.214202301601447 | 0.79908041 | -0.060052779 | -0.070257122 |
| 29 | 0.214292070528504 | 0.214292070528505 | 0.79908041 | 0 | 0 |
| 30 | 0.216229121969610 | 0.216229121969622 | 0.79908041 | 0 | 0 |
| 31 | 0.217852393265892 | 0.217852393265904 | 0.79908041 | -0.060052779 | -0.070257122 |
| 32 | 0.224831328559860 | 0.224831328559860 | 0.79908041 | -0.055770202 | -0.053044309 |
| 33 | 0.251790018203106 | 0.251790018203106 | 0.633410887 | 0 | 0 |
| 34 | 0.254871326636724 | 0.254871326636729 | 0.633410887 | -0.007088203 | -0.014227501 |
| 35 | 0.299021704854000 | 0.299021704854004 | 0.633410887 | 0 | 0 |
| 36 | - | - | 0.633410887 | - | - |

TABLE II. Permanent and transition dipole elements of first four singlet states. Comparison between our theory, Eq. (55), and Full MRCI (reference). Resymmetrization values included. All values are reported in atomic units.

Our theory, Eq. (55)

| $\langle\Psi_I\|\hat{D}\|\Psi_J\rangle$ | 0 | 1 | 2 | 3 |
|---|---|---|---|---|
| 0 | 0.280450545531325 | 0.327160067460011 | 0.359364595066135 | 0.280648617707319 |
| 1 | 0.327160067459790 | -0.032500798288387 | 0.186908801797801 | -0.023390872061993 |
| 2 | 0.359364595066199 | 0.186908801798012 | 0.018980615290030 | 0.171564525533033 |
| 3 | 0.280648617707139 | -0.023390872061909 | 0.171564525533258 | 0.006223527692625 |

Full MRCI (reference)

| $\langle\Psi_I\|\hat{D}\|\Psi_J\rangle$ | 0 | 1 | 2 | 3 |
|---|---|---|---|---|
| 0 | 0.280450545531200 | 0.327160067459983 | 0.359364595066106 | 0.280648617707180 |
| 1 | 0.327160067459983 | -0.032500798288235 | 0.186908801797968 | -0.023390872061930 |
| 2 | 0.359364595066106 | 0.186908801797968 | 0.018980615290055 | 0.171564525533220 |
| 3 | 0.280648617707180 | -0.023390872061930 | 0.171564525533220 | 0.006223527692478 |

$\tilde{r}_{IJ}$ matrix, Eq. (48)

| $\tilde{r}_{IJ}$ | 0 | 1 | 2 | 3 |
|---|---|---|---|---|
| 0 | 1.000000000000000 | 1.019356578034540 | 1.001460871475910 | 1.004584129450090 |
| 1 | 0.981010984329088 | 1.000000000000000 | 0.982444115293655 | 0.985508065673220 |
| 2 | 0.998541259556388 | 1.017869601367700 | 1.000000000000000 | 1.003118701951450 |
| 3 | 0.995436788900292 | 1.014705038783090 | 0.996890994111274 | 1.000000000000000 |

## II. ADDITIONAL RESULTS

**Effect of modifying $U/t$ ratio**.

The model is sensitive to the $U/t$ ratio. For example, if $t$ is slightly lowered to 0.125 eV, the following profiles are obtained:

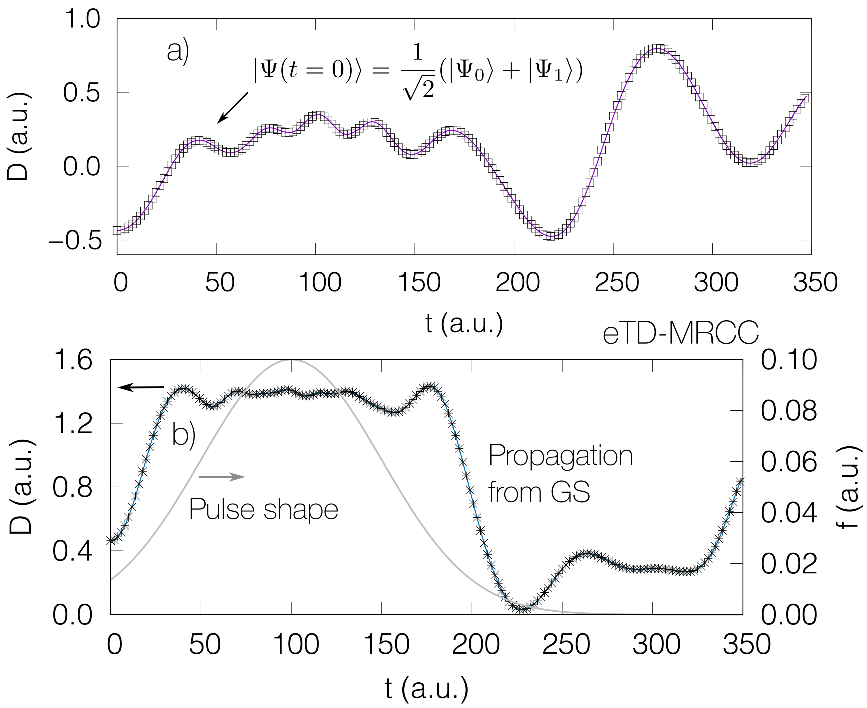


FIG. 1. Time dependency of observable $\hat{D}$. Solid lines: eTD-MRCC, symbols: numerically exact, reference, unitary propagation. a) Propagation from coherent initial state, b) propagation from GS, perturbating pulse shown in b) as well.

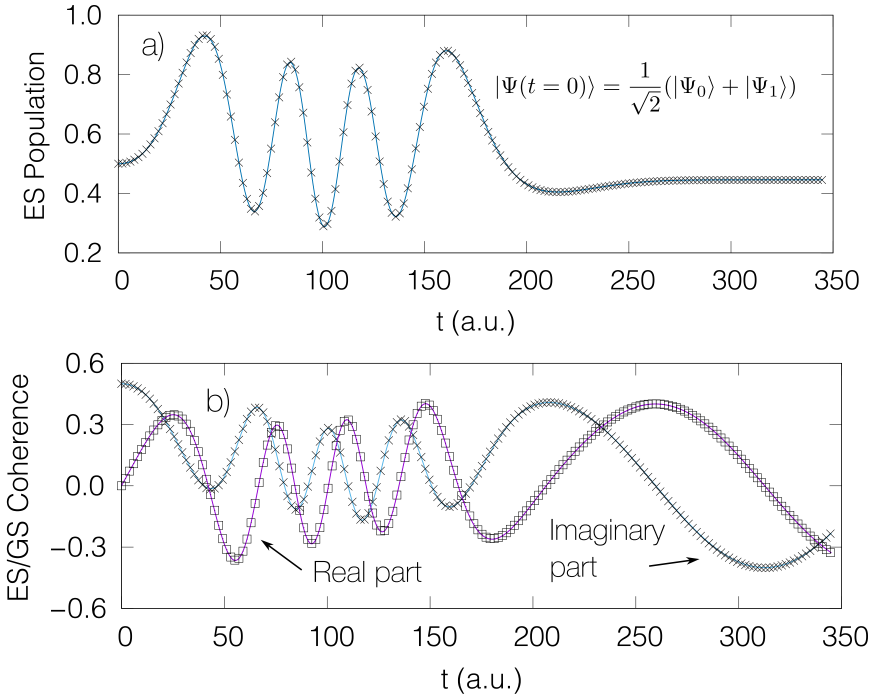


FIG. 2. Excited state (first singlet $|\Psi_1\rangle$) TD probability and coherence. Solid lines: eTD-MRCC, symbols: numerically exact, reference, unitary propagation.

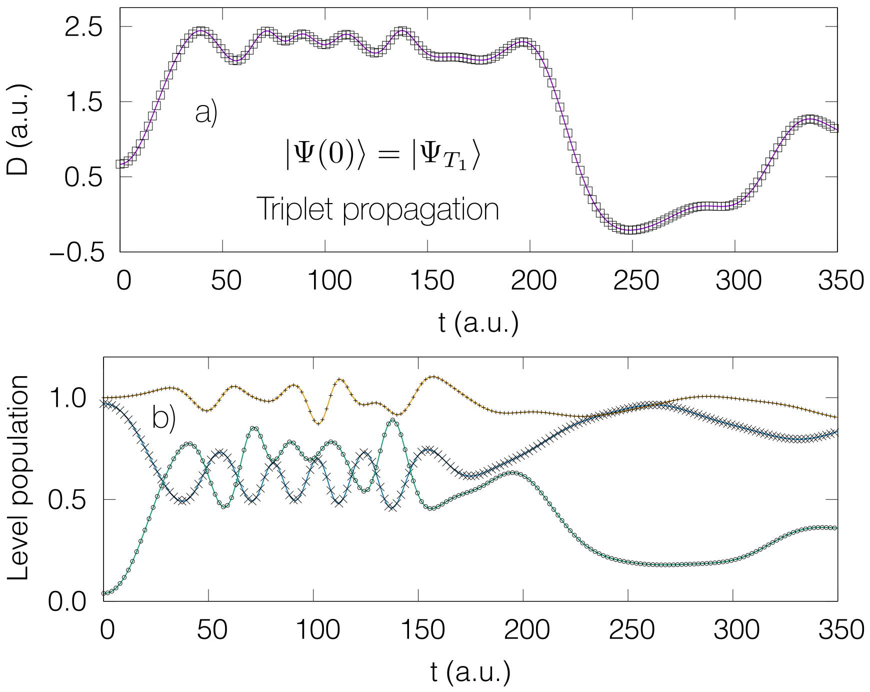


FIG. 3. Time-dependent dipole for propagation from lowest-energy triplet state. Solid lines: eTD-MRCC, symbols: numerically exact, reference, unitary propagation.
